# Supplementary material for: Radiation reaction cooling as a source of anisotropic momentum distributions with inverted populations
Source: arXiv:2212.12271 source file (2023-03-29)
Supplement: Supplementary file 1 [file supplemental.tex]

\documentclass[%
onecolumn,
%twocolumn,
%superscriptaddress,
%groupedaddress,
%unsortedaddress,
%runinaddress,
%frontmatterverbose, 
%preprint,onecolumn,
%preprintnumbers,
%nofootinbib,
%nobibnotes,
%bibnotes,
 amsmath,amssymb,
 %aps,
 prl,
%pra,
%prb,
%rmp,
%prstab,
%prstper,
%floatfix,
]{revtex4-2}
\usepackage{graphicx}% Include figure files
\usepackage{xcolor}
\begin{document}
\title{Supplemental material for Synchrotron cooling as a source of momentum distributions with inverted Landau populations}
\maketitle

\input{supplemental/supplemental_text.tex}
%\newpage
%\bibliography{apssamp}

\end{document}
